# Supplementary material for: Optically coherent nitrogen-vacancy centers in {\mu}m-thin etched diamond membranes
Source: arXiv:1904.00883 ancillary file (2019-04-01)
Supplement: Supplementary file 1 [file supplement_arxiv.pdf]

# Supplementary information: Optically coherent nitrogen-vacancy centers in µm-thin etched diamond membranes

Maximilian Ruf,[1,2,*] Mark IJspeert,[1,2,3,*] Suzanne van Dam,[1,2]
Nick de Jong,[1,4] Hans van den Berg,[1,4] Guus Evers,[1,2] and Ronald Hanson[1,2,†]

[1] *QuTech, Delft University of Technology, 2628 CJ Delft, The Netherlands*
[2] *Kavli Institute of Nanoscience, Delft University of Technology, 2628 CJ Delft, The Netherlands*
[3] *Current address: Clarendon Laboratory, Parks Road, Oxford OX1 3PU, United Kingdom*
[4] *Netherlands Organisation for Applied Scientific Research (TNO), 2628 CK Delft, The Netherlands*

## I. DIAMOND SURFACE EVOLUTION UNDER ICP-RIE ETCHING WITH $SF_6$ AND AR/$CL_2$

This section describes the systematic study of the evolution of diamond surfaces on the microscopic level under reactive ion etching (RIE) using an inductively coupled plasma (ICP). All measurements were performed on high pressure, high temperature (HPHT) grown, $\langle 1\,0\,0\rangle$ oriented type Ib diamonds (Element Six, 3 × 3 × 0.3 mm). These diamonds contain many surface and subsurface defects resulting from the growth and polishing process. When excluding these defect areas intrinsic to HPHT samples, this material can still be used to extract quantitative surface data when comparing different processing steps (see sections below).

### A. Sample preparation

Before etching, as-received HPHT diamonds are cleaned in $HNO_3$ (99%) for 10 minutes. The samples are then rinsed for 10 minutes in de-ionized (DI) water, cleaned in acetone in an ultrasonic bath for 5 minutes, rinsed for one minute in isopropyle alcohol (IPA), and blow-dried with nitrogen.

During this research, we have compared the effect of different pre-etch wet cleaning methods on the diamond surface quality after etching. While we have not compared the number of particles after different wet cleaning methods quantitatively, we find that the $HNO_3$ cleaning described above yields a similar surface roughness after etching in comparison with commonly used, yet time-consuming techniques such as tri-acid and hydrofluoric acid (HF).

### B. Diamond etching methods

Etch procedures were carried out using ICP-RIE (Oxford Plasmalab 100). Many holes are formed during etching of diamond surfaces when using etch holders made out of Si or $Al_2O_3$, as the respective material is etched and re-deposited. Following the same mechanism as reported in the main text, this leads to hole formation in the diamond surface. To avoid this process, we use a 4 inch fused quartz carrier wafer during etching, that shows minimal material re-deposition on the diamond surface. To avoid charging during etching (which prevents the release of the carrier wafer from a mechanically clamped wafer holder after etching), we apply a $\sim$ 15 nm thick Ti layer on the backside of this wafer via sputter deposition (Alliance Concept AC450), and clamp the wafer in the etcher with a metal ring. A summary of all etch parameters and measured etch rates (diamond sample and fused quartz carrier wafer) can be found in Table I.

### C. Atomic Force Microscopy analysis

The Atomic Force Microscope (AFM, Bruker FastScan) data underlying the evolution of the height of a particle w.r.t. the mean diamond surface height for identical areas and different etch times as displayed in Fig. 3 of the main text can be seen in Fig. 1 for the $SF_6$ based etching sequence, and in Fig. 2 for the Ar/$Cl_2$ based etching sequence. We infer the particle heights and errorbars by plotting a histogram of surface height around a particle, and taking the mean and standard deviation of the distribution after employing a cut-off above the mean sample surface height.

| | $O_2$ | Ar/$Cl_2$ | $SF_6$ |
|---|---|---|---|
| ICP / RF power (W) | 1100 / 90 | 500 / 200 | 500 / 50 |
| Gas flow (sccm) | 50 $O_2$ | 10 Ar / 20 $Cl_2$ | 30 $SF_6$ |
| Pressure (µbar) | 10 | 10 | 13 |
| Carrier wafer temperature (°C) | 20 | 30 | 30 |
| Diamond etch rate (masked, nm/min) | 210 ± 10 | 42 ± 2 | Unmeasured |
| Diamond etch rate (not masked, nm/min) | 350 ± 20 | 39 ± 2 | 44 ± 2 |
| Fused quartz etch rate (nm/min) | 11 ± 1 | 80 ± 5 | 113 ± 6 |

TABLE I. Summary of etch parameters and diamond sample and fused quartz carrier wafer etch rates found in this work.

| | $Ar/Cl_2$ time (min) | $O_2$ time (min) | Thickness $t_m$ (μm) |
|---|---|---|---|
| Before any etching | – | – | 47.8 ± 0.2 |
| First etching step | 26 | 45 | 37.7 ± 0.2 |
| Second etching step | 30 | 138 | 10.1 ± 0.2 |
| Third etching step | 30 | 23 | 3.8 ± 0.2 |

TABLE II. Summary of etching times under $Ar/Cl_2$, followed by $O_2$, and corresponding thickness in NV measurement region $t_m$ after each etching step, measured with a stylus profilometer.

## II. FABRICATION OF A THIN DIAMOND PLATELET

This section describes the full process-flow employed to fabricate the (3.4 ± 0.2) μm thick diamond plate discussed in the main text.

We start fabrication by irradiating as-received, commercially available type IIa CVD grown diamonds (Element Six, 2 × 2 × 0.5 mm, company specified nitrogen density < 885 $\mu m^{-3}$, $\langle 1\,0\,0 \rangle$ crystal orientation) with electrons (electron energy 2 MeV, fluence 1 or 5× $10^{13}$ $e^-/cm^2s$) at the Reactor Institute in Delft. As described in the main text, this forms vacancies in the diamond lattice (∼ 30 or 150 $\mu m^{-3}$). On samples that underwent the same procedure as the one described here, we find typical natural NV density values of < 0.005 $\mu m^{-3}$ (compared to company specified values of < 5 $\mu m^{-3}$). To reduce potential diamond surface contamination with metals resulting from the diamond polishing process [1, 2] that could lead to contamination of the annealing chamber, we immerse the samples in a mixture of 1:1:1 $H_2SO_4$(97%):$HNO_3$(60%):$HClO_4$(60%) at 120 °C for one hour in a re-flux configuration. We then rinse the sample for 10 minutes in de-ionized (DI) water, clean it for 5 minutes in acetone in an ultrasonic bath, rinse it for one minute in isopropyl alcohol (IPA), and blow-dry the sample with nitrogen.

Next, we anneal the sample in a three step high temperature annealing process under high vacuum (< $10^{-6}$ mbar) to combine vacancies with naturally occurring nitrogen in the sample to form NV centers, and to anneal out defects such as di-vacancies [3]. We ramp the temperature from room temperature to 400 °C in 4 hours, hold the temperature constant for 8 hours, increase the temperature to 800 °C over a 12 hour time-span, hold this temperature for 8 hours, increase the temperature to 1100 °C in 12 hours, hold it constant for a period of 10 hours, and then switch off the oven to cool to room temperature. All temperature increases are ramped linearly at a slow rate to maintain a high vacuum in the annealing chamber that is needed to avoid surface graphitization of the diamond [3]. This treatment results in typical NV densities of (0.01 - 0.1) $\mu m^{-3}$.

After slicing of a sample into three membranes of ∼ 50 μm each, the membranes are polished to a surface roughness of typically $r_q$ < 1 nm (Delaware Diamond Knives). We then clean the membranes in $HNO_3$ (99%) for 10 minutes, followed by the same after-acid cleaning and drying procedure as described above. Subsequently, we bond the sample via Van der Waals forces to a mirror patterned with golden markers and strip lines to allow for repeated localization of the same area in subsequent NV characterization steps, and for application of microwaves to NV centers [4] .

As discussed in the main text, the exposure of mirror material to the plasma leads to severe micromasking on the diamond. We therefore mask the diamond and mirror from the top with a fused quartz wafer (thickness 500 μm) that has a laser-cut square opening (Lasertec BV) (1.4 mm side length on the side facing the diamond, narrowing towards the top at an angle of 30 ° to reduce etch-induced trenching effects [5], see Fig. 4 of the main text for mask geometry). This prevents exposure of mirror material to the etching plasma. We then etch the diamond in different ICP-RIE steps as described in the main text and summarized in Table II, using the plasma parameters summarized in Table I. Note that once bonded, we do not wet-clean the sample in between etch steps.

## III. NV CHARACTERIZATION METHODS

### A. Experimental setup

To measure the optical properties of NV centers, we use a home-built confocal microscope operated at low temperature (< 10 K) inside a closed-cycle cryostat (Montana Instruments s50) with optical access. A microscope objective (Olympus MPLFLN-100X) is mounted on an xyz scanner (Physik Instrumente P-615K011). To extract the NV transition linewidths, we lock a 637 nm external cavity laser (New Focus Velocity TLB-6700) to a wavemeter (High finesse WS-6) via a PC controlled PID loop acting on the laser control. We then sweep the setpoint of the lock, and detect fluorescent photons from the NV emitted in the phonon side band (PSB) on an APD (Laser Components Count-20C-FC), while

* These authors contributed equally to this work.
† r.hanson@tudelft.nl

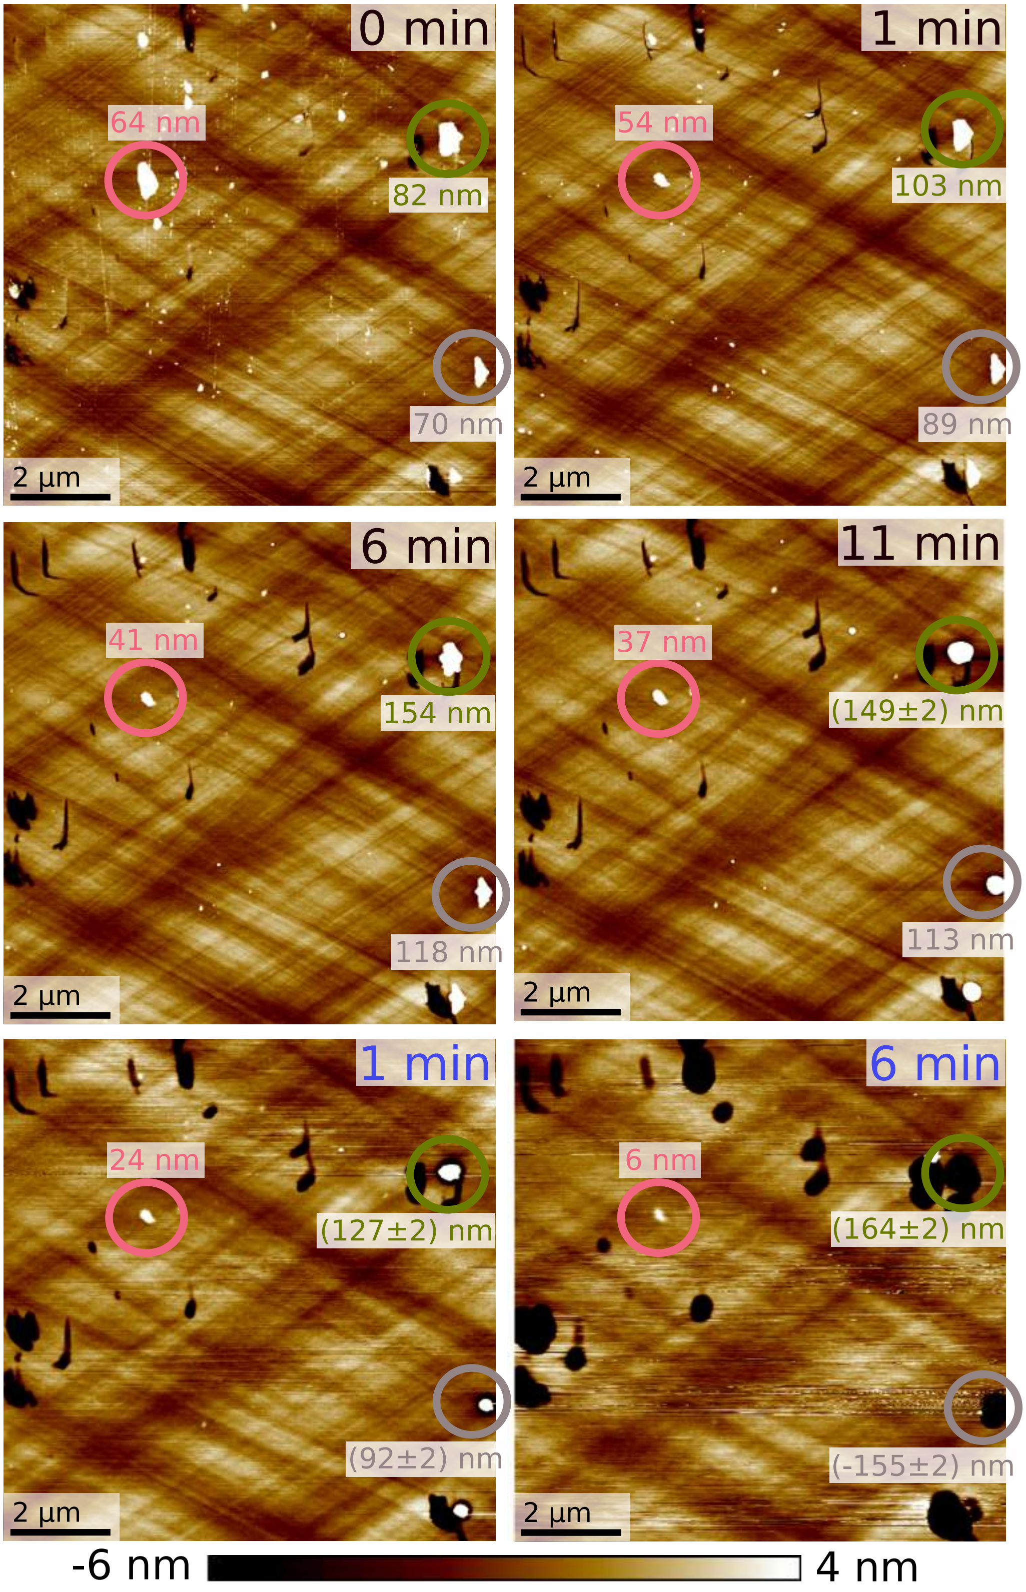


FIG. 1. Evolution of an identical HPHT diamond surface area during ICP-RIE with $SF_6$ (black time indication), followed by etching with $O_2$ (blue time indication), for different etching times (indicated in the top right of each AFM trace). This sample shows many surface defects, resulting from the diamond growth and polishing process. Colored circles indicate the relative height of particles w.r.t. the mean diamond surface height for a specific etch time, with an errorbar of $\pm1$ nm unless otherwise indicated. This data underlies Figure 3 of the main text.

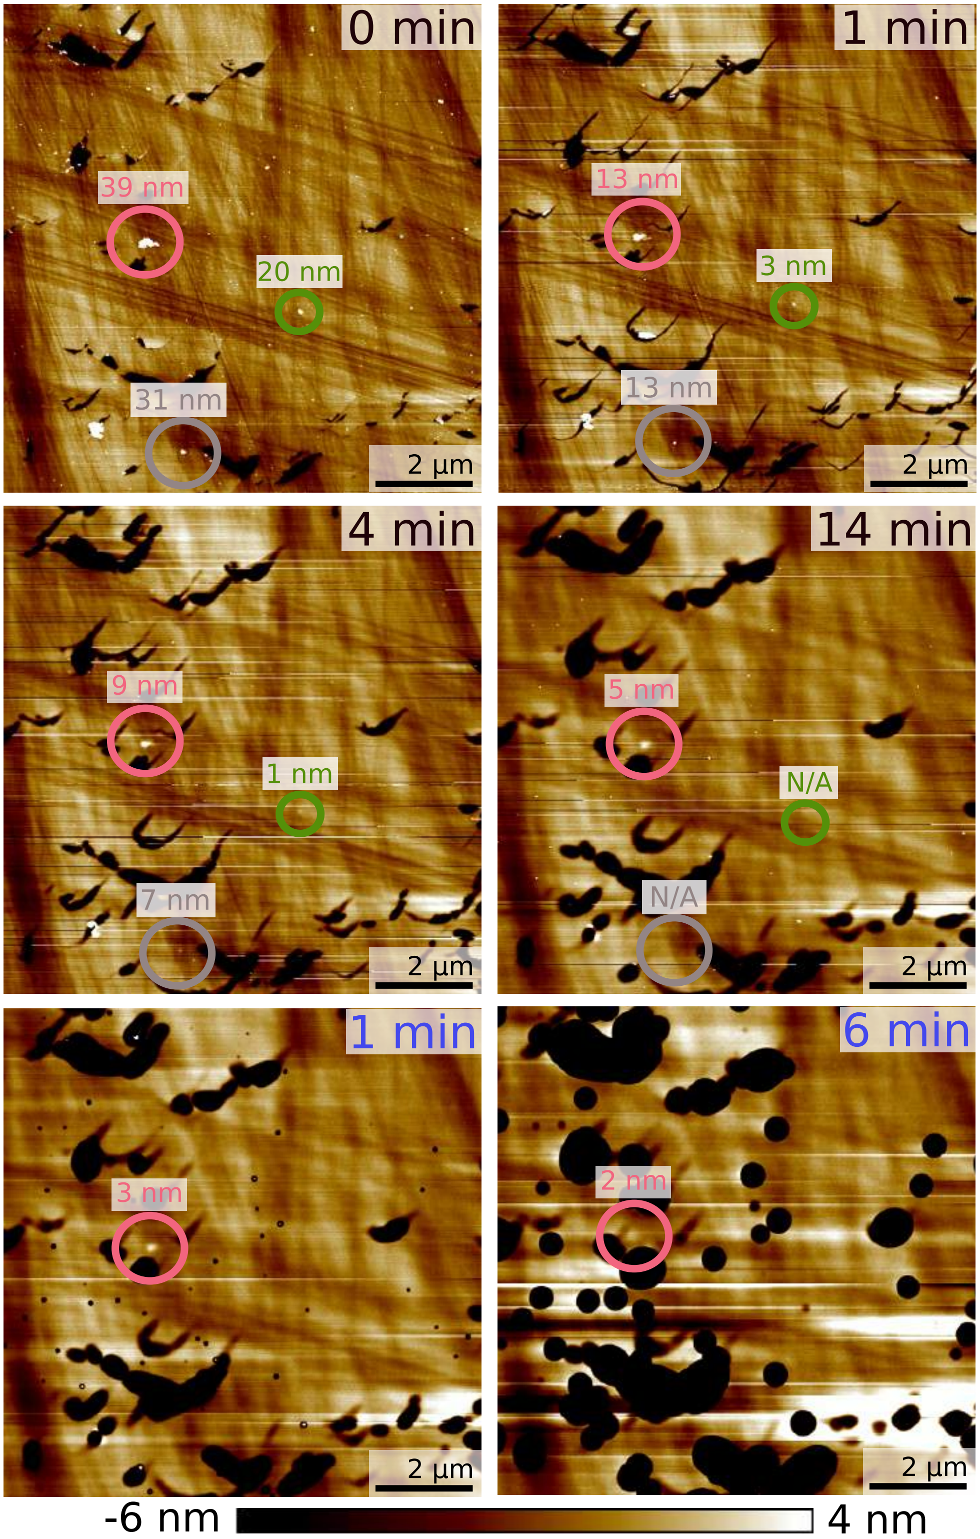


FIG. 2. Evolution of an identical HPHT diamond surface area during ICP-RIE for different etching times (indicated in the top right of each AFM trace) with Ar/$Cl_2$ (black time indication), followed by etching with $O_2$ (blue time indication). This sample shows many surface defects, resulting from the diamond growth and polishing process. Colored circles indicate the relative height of particles w.r.t. the mean diamond surface height for a specific etch time, with an errorbar of $\pm 1$ nm. Note that for this particular etch sequence, many particles are introduced by handling the diamond in between etch steps (e.g. visible by comparing the images after 1 min and 14 min of Ar/$Cl_2$ etching). This explains the formation of many small holes after 1 min of $O_2$ etching, that can be avoided when etching directly after the Ar/$Cl_2$ etch (i.e. without unloading the diamond from the etcher). This data underlies Figure 3 of the main text.

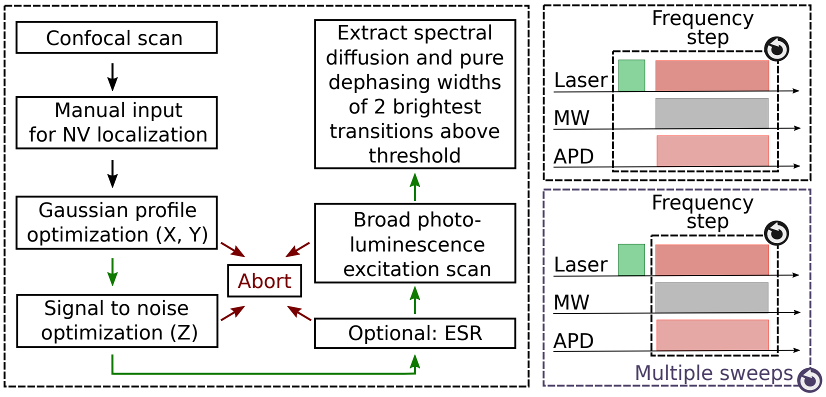


FIG. 3. Sketches of automated data acquisition sequence and employed laser scans. (Left) Decision tree employed during automated data acquisition. Black arrows indicate that no software decision is made, green arrows represent continuation after a positive previous step, and red arrows indicate that the previous step failed, the routine is aborted, and the software starts over with a Gaussian profile optimization at potential NV center locations (see text for detailed description of each step). (Right, top) Schematic of the pulse sequence used during a broad PLE scan. Green laser pulses (10 μW, 10 μs) are continuously interleaved with red laser pulses (20 nW, 100 μs, with a wait time of 10 μs in between pulses), while sweeping the red laser's frequency with a resolution of 10 MHz, and integrating for a total time of 25 ms per frequency point. (Right, bottom) Schematic of the pulse sequence used to characterize an individual NV center ZPL line. In contrast to the sequence employed in (right, top), we only apply one green pulse (10 μW, 1s) at the beginning of each red frequency sweep. We then sweep the red laser's frequency (8 nW) with a resolution of 4 MHz, and integrate for 10 ms per point.

recording the corresponding laser frequency value. The PSB is spectrally separated from the zero phonon line by a dichroic mirror (Semrock L2NL-0016) with a custom made razor edge at $\sim 637$ nm. We use off-resonant green laser excitation (532 nm, Cobolt Samba 100) to initialize the NV in the negative charge state and $m_s = 0$ spin state. The laser pulses are created via acousto-optic modulators (Gooch and Housego). To further suppress unwanted residual light from the green laser, we introduce an additional PC-controlled home-built shutter in the beam path after the second round of measurements of Fig. 5 in the main text (i.e. starting from measurements after the second membrane etch). To rotate the NV electron spin, we generate microwave signals via an arbitrary waveform generator (AWG) and a microwave source (Rhode und Schwarz SMBV100A) that are amplified (Amplifier Research 40S1G4) before delivery to the striplines on the mirror.

## B. Data acquisition sequence

We have developed a largely automized software sequence that allows us to measure the spectral diffusion and dephasing linewidths of many NV centers. An overview of the decision tree followed is displayed in Fig. 3 (Left).

### 1. *NV localization*

After performing a confocal microscope scan ($\lambda = 532$ nm, see Fig. 4 (A) for an example), potential NV center locations are selected via manual input. If one dimensional off-resonant scans ($\lambda = 532$ nm) along both the x- and y- directions show a fluorescence profile with a Gaussian profile within certain width bounds after a maximum of 3 optimizations each, the protocol continues by optimizing the signal to noise ratio of a scan along the x-direction for different z positions of the objective. This method allows to determine the optimal focal distance, as it does not take into account background fluorescence originating from defects in the mirror substrate. We then measure a continuous wave (CW) optically detected magnetic resonance spectrum (ODMR) around the NV zero field splitting ($\approx 2.88$ GHz, see Fig. 4 (B)). As the quality of the microwave striplines deteriorates after prolonged etching, ODMR scans are only performed for the first two sets of data. If a dip in the fluorescence signal (corresponding to the $m_s = 0$ to $m_s = 1$ spin transition) falls below one standard deviation from the data mean, we mark the spot as a potential NV center and continue with characterization of the optical transition frequencies. For all subsequent measurements, we use either the microwave frequency found by fitting the CW-ODMR spectra, or the zero field splitting frequency of 2.88 GHz (starting from the third set of data, from which on reduced microwave stripline quality does not allow us to detect CW-ODMR signals).

### 2. *Optical characterization*

We proceed with scanning a tuneable laser around the expected ZPL transition wavelength, while detecting photons emitted from the NV in the phonon side

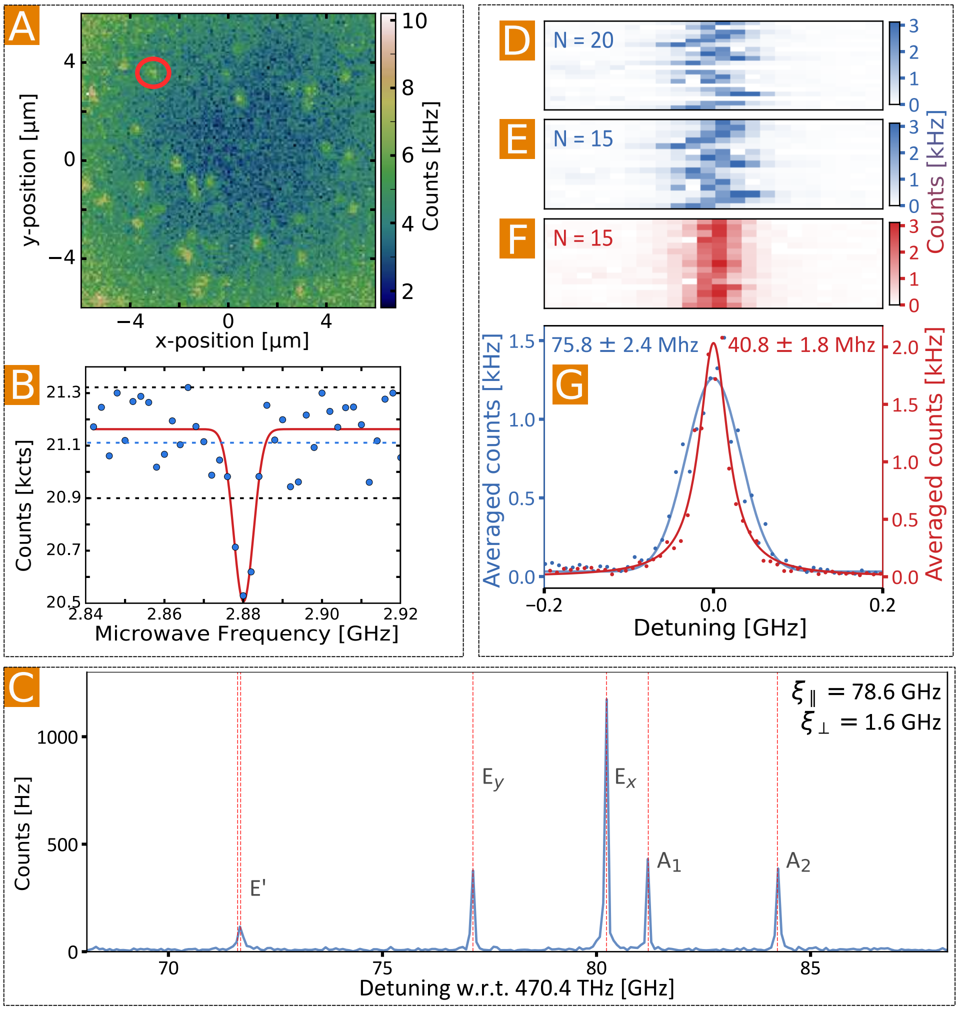


FIG. 4. Examples of measurement results during data acquisition for one NV center. (A) Confocal microscope scan under green excitation ($\lambda = 532$ nm), with the NV measured throughout this figure encircled in red. (B) Optically detected magnetic resonance of the NV center ($\lambda = 532$ nm) under no external magnetic field, with the mean of the datapoints and one standard deviation from the mean labeled in red and blue, respectively. Since a dip in the fitted ESR spectrum corresponding to the $m_s = 0$ to $m_s = \pm 1$ spin transitions deviates more than one standard deviation from the mean, the routine continues with a PLE scan at this position. (C) PLE of the ZPL lines, showing six lines associated with the allowed optical transitions of the NV center from the ground to the excited state. Note that the $E_1$ and $E_2$ transitions overlap and are labeled as $E'$. Red lines correspond to transition energies calculated from the NV Hamiltonian, using the $m_s = 0$ transition frequencies ($E_x$ and $E_y$) as inputs to the model. (D) Series of 20 PLE scans of the $E_x$ transition displayed in (C), binned into 8 MHz frequency steps. Spectral jumps due to green repump pulses and empty traces due to NV center ionization are visible. (E) Remaining 15 PLE traces of the data displayed in (D) after removal of ionized traces, giving an indication of the spectral diffusion width of the individual ZPL transition. (F) Data displayed in (E), with fitted lorentzian center frequencies of individual traces used to align frequency axes to each other, to reveal the dephasing linewidth of the ZPL transition. (G) (Blue) Averaged and gaussian fitted data of (E), revealing a Gaussian spectral diffusion linewidth of (75.8 ± 2.4) MHz. (Red) Averaged and Lorentzian fitted data of (F), yielding a dephasing linewidth of (40.8 ± 1.8) MHz.

band (PSB, see Fig. 4 (C)). To detect all six allowed spin-conserving ZPL transitions, we constantly apply microwaves to mix the NV spin levels, while interleaving pulses of the tuneable red laser with green laser pulses to ensure the NV is in the negative charge state via optical off-resonant pumping, see Fig. 3 (Right, top). The software then selects the brightest peaks above a certain threshold (maximum of 2 peaks) for a narrow linescan. In this case, it repeatedly applies a sequence of a short green laser pulse (to ensure spin and charge state initialization), followed by a red frequency sweep through the expected transition frequency (to map out the specific ZPL transition under dephasing). This is done while constantly applying microwaves to avoid pumping in an optically dark spin state, see Fig. 3 (Right, bottom). Fig. 4 (D) shows an example of 20 subsequent scans conducted in this manner, with spectral jumps resulting from a changing charge state distribution in the NV

vicinity and empty traces due to photo-ionization visible. We then remove photo-ionized traces, and obtain the NV linewidth under spectral diffusion (via a gaussian fit to the averaged counts of all scans, see Fig. 4 (E)), as well as the full width at half maximum (FWHM) of the average dephasing linewidth. To extract all dephasing linewidth data shown in this manuscript, we fit each line profile individually, and calculate the weighted average, $\gamma$, for all scans of a certain transition via

$$\gamma = \frac{\sum_i \gamma_i \sigma_i^{-2}}{\sum_i \sigma_i^{-2}}, \qquad (1)$$

where $\gamma_i$ is the FWHM of an individual lorentzian shaped trace, and $\sigma_i$ the corresponding standard error of the fit. The errorbar of the average dephasing linewidth, $\sigma_\gamma$, is then given by

$$\sigma_\gamma = \sqrt{\frac{1}{\sum_i \sigma_i^{-2}}}. \qquad (2)$$

Fig. 4 (F) shows the results of the 15 remaining scans displayed in Fig. 4 (E) after aligning the center frequency of each fitted trace, to show the effect of dephasing. Fig. 4 (G) shows the averaged counts of the traces in Figs. 4 (E) and (F) in blue and red, respectively. The solid blue and red lines indicate a Guassian and Lorentzian fit to this data, respectively. Note that the way of extracting the dephasing linewidth in this figure by fitting one lorentzian to the averaged data is different from the approach described above and used in the rest of this paper, which is based on fitting all linescans individually, and calculating their weighted mean. Fitting the averaged data is chosen here for ease of visualization.

## IV. LASER-POWER INDUCED LINEWIDTH BROADENING

To quantify the contribution of laser-power induced linewidth broadening to the measured dephasing linewidths, we model each ZPL transition as an ideal two-level system [6, 7]. Following this model, we fit the theoretically expected curve of form $\sqrt{\gamma_i^2 + \Omega^2}$ to our data, where $\gamma_i$ is the natural linewidth of the NV transition, and $\Omega^2 = b \times P$ the squared Rabi frequency, where $P$ is the applied laser power and $b$ is a constant. We scan a laser twenty times over a pre-localized NV transition (using the pulse sequence described above and depicted in Fig. 3 (Right, bottom)), and extract the weighted average dephasing linewidth (as described above). We repeat this measurement for different powers of the red laser beam. Fig. 5 shows the result of the fit. We extract a natural dephasing linewidth of (18.3 $^{+5.7}_{-8.7}$) MHz, compared to an extracted FWHM of (48.7 $\pm$ 0.7) MHz when using 8 nW of red power, as used throughout this paper. This means that the transition is power broadened, potentially explaining why we do not observe lifetime-limited linewidths throughout this paper.

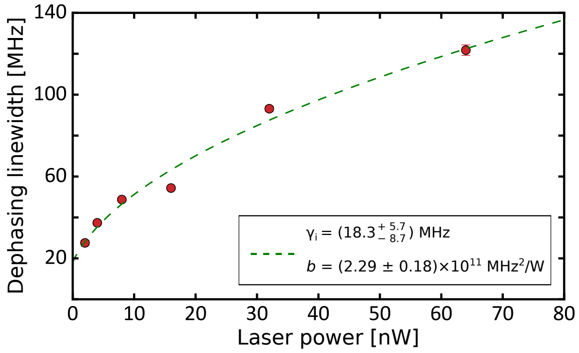


FIG. 5. Dephasing linewidth as a function of laser power (solid red datapoints), and corresponding fit (green dashed line, see text for description). Throughout this paper, 8 nW of red power were used to measure the dephasing linewidths of NV centers, resulting in operation in the power broadening regime.

## V. OBJECTIVE DEPTH CONVERSION FACTOR

The high refractive index of diamond leads to a shift in the observed focal point position w.r.t. that in vacuum. We determine the resulting conversion factor between distance travelled by the microscope objective and distance travelled by the focal point in diamond in the following way: we first measure the distance $t_f$ which we need to shift our microscope objective to move the laser focus from one diamond surface to the other, i.e. from the air-diamond to the diamond-mirror interface. We then determine the inverse ratio of this value and the actual diamond thickness as measured by a stylus profilometer. Table III displays the data obtained in this way. By evaluating the propagation of the uncertainties on the individual values, we obtain an average conversion factor of $2.64^{+0.11}_{-0.09}$ for our dataset. Throughout this paper, we use this conversion factor to determine the depth of NV centers w.r.t. the mirror interface. This is the reason for the discrepancy of the thicknesses indicated by the color shading in Fig. 5 of the main text compared to the directly reported values of diamond thicknesses in the measurement region that have been directly obtained by stylus profilometer measurements.

## VI. CONFOCAL NV DEPTH ERROR ANALYSIS AND DUPLICATE REMOVAL

In order to estimate the error on the depth of an NV center as determined by the method described above, we plot a histogram of the frequency difference between all measured NV center peaks, as displayed in Fig. 6 (A). A peak around a frequency difference of zero, that results from scanning a given NV center twice, is visible. This can happen for our scans, as the focal depth in our setup broadens with increasing distance from the diamond sur-

| | Diamond thickness | Objective travel distance | Conversion factor |
|---|---|---|---|
| | $t_m$ (µm) | $t_f$ (µm) | |
| Before any etching | 47.8 ± 0.2 | 18.2 ± 0.2 | $2.63^{+0.04}_{-0.04}$ |
| First etching step | 37.7 ± 0.2 | 14.6 ± 0.2 | $2.58^{+0.05}_{-0.05}$ |
| Second etching step | 10.1 ± 0.2 | 3.4 ± 0.2 | $2.97^{+0.25}_{-0.22}$ |
| Third etching step | 3.8 ± 0.2 | 1.6 ± 0.2 | $2.38^{+0.48}_{-0.38}$ |

TABLE III. Summary of diamond membrane thicknesses as measured with a stylus profilometer, corresponding objective travel distance, measured by determining the separation between focusing on the two diamond surfaces (i.e. the air-diamond and diamond-mirror interfaces), and resulting calculated conversion factors.

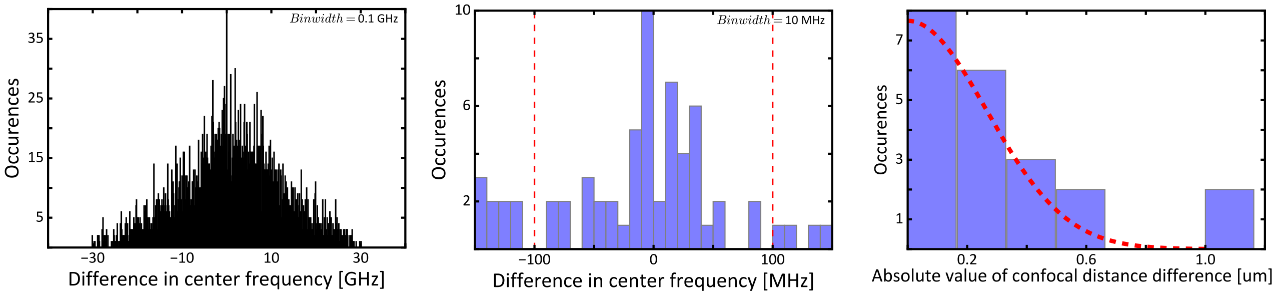


FIG. 6. Estimation of confocal NV depth errorbar. (A) Histogram of difference between center frequencies of all measured NV center peaks, binned into 0.1 GHz bins. A peak around zero frequency difference that we attribute to repeated scanning of identical blobs is visible. (B) Histogram of difference between center frequencies of all measured NV center peaks, binned into 10 MHz bins, zoomed in to a range from -150 MHz to 150 MHz. Dotted red vertical lines denote used frequency bounds for (C) Histogram showing absolute values of confocal distance difference of blobs that are likely identical. Red dotted line denotes fit result to a Gaussian function (see text for functional form). The datapoints are found using the frequency criterion displayed in (B), and the requirement that the Euclidean distance between NVs that this frequency difference results from is less than (4 µm)$^3$.

face (see section V). As a consequence, the bright fluorescence profile of a single NV center can appear at various objective positions. Additionally, some NV centers are close to each other, which triggers the position optimization algorithm to select the same NV center in different scans. We use this information about blobs likely to be the same to remove double entries: if the peak frequencies of two seperately measured NV centers differ by less than 100 MHz (see Fig. 6 (B)), and if the Euclidean distance between those NV centers is less than (4 µm)$^3$, we consider these NVs to be the same, and only keep the data for one of them in our analysis. We also use this criterion to extract the depth error from multiple measurements on identical NV centers: the first step is to consider the absolute difference $Z$ in confocal depth for both of such measurements. This difference can be defined as $Z := X_1 - X_2$, where the first and second measurements are realizations of the independent random variables $X_1, X_2 \sim \mathcal{N}(\mu, \sigma^2)$ respectively, where $\mathcal{N}$ is the normal distribution with mean $\mu$ and standard deviation $\sigma$. The idea is to extract $\sigma$ from the explicit form of the probability density function that governs the random variable $|Z|$. First note that $Z \sim \mathcal{N}(0, 2\sigma^2)$. Thus, for $x \geq 0$, the cumulative distribution function $F_{|Z|}(x)$ can be written as:

$$\begin{aligned} F_{|Z|}(x) &:= P(|Z| \leq x) \\ &= P(-x \leq Z \leq x) \\ &= P(-x < Z \leq x) \\ &= F_Z(x) - F_Z(-x) \\ &= 2F_Z(x) - 1\,. \end{aligned}$$

Note that $F_{|Z|}(x) = 0$ for $x < 0$, such that the probability density function $f_{|Z|}(x)$ now equals:

$$\begin{aligned} f_{|Z|}(x) &:= \frac{\partial}{\partial x} F_{|Z|}(x) \\ &= 2 f_Z(x) \mathbb{1}_{(0,\infty)}(x) \\ &= \frac{1}{\sigma\sqrt{\pi}} \exp\left(-\frac{x^2}{4\sigma^2}\right) \mathbb{1}_{(0,\infty)}(x)\,, \end{aligned}$$

where $\mathbb{1}_{(0,\infty)}$ is the Heaviside step function. Fitting this functional form to the data displayed in Fig. 6, we extract an errorbar of 0.18 µm for our dataset. Assuming this error to be independent from the error we determined for the conversion factor (see Sec. V), we calculate the root sum of squared uncertainties to determine the overall uncertainty of the distance of an NV center from the diamond-mirror interface for all datapoints in this paper.

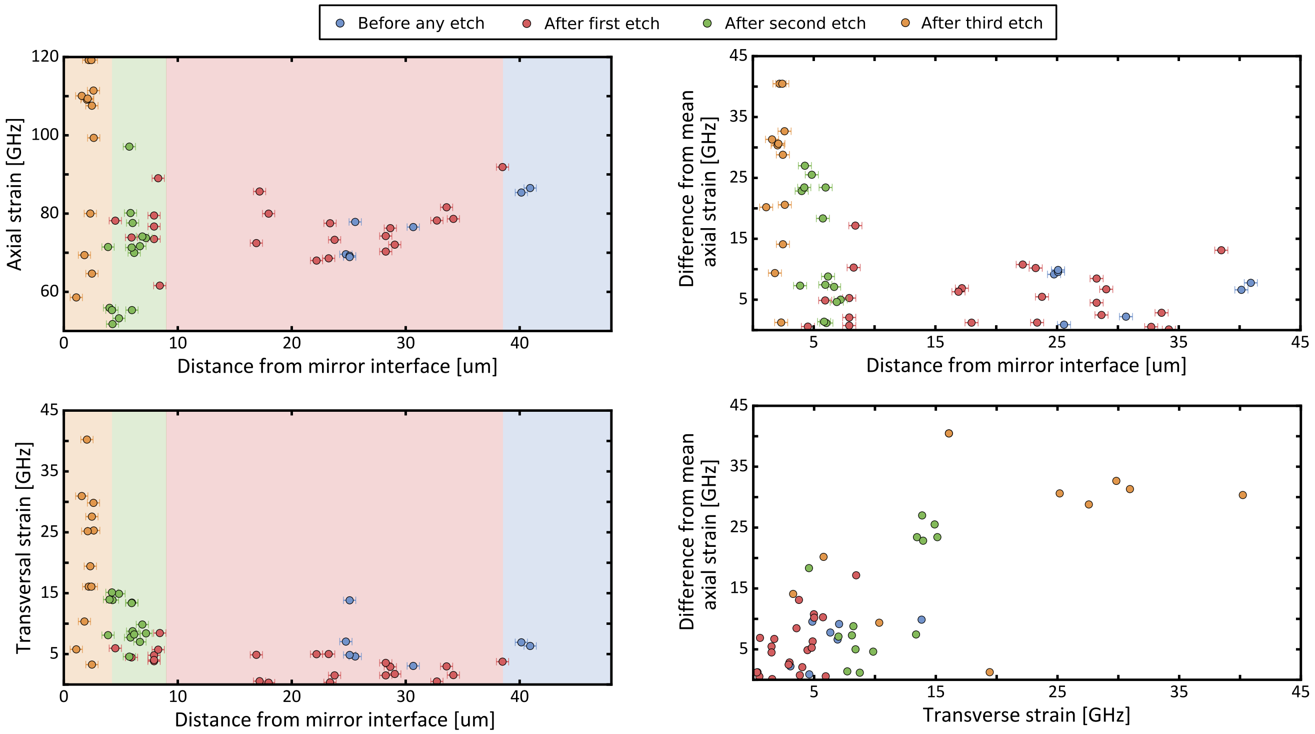


FIG. 7. Dependence of axial and transverse strain on the NV distance from the diamond-mirror interface and dependence of axial on transverse strain for these NVs. (Left, top) Dependence of total axial strain (w.r.t. 470.4 THz) on the mirror interface distance. (Left, bottom) Transverse strain as a function of mirror interface distance. (Right, top) Dependence of the difference of axial strain of individual NVs and the mean of axial strains of the whole dataset on the mirror interface distance. (Right, bottom) Dependence of the difference of axial strain of an individual NV and the mean of axial strains of the whole dataset on transverse strain. (Blue) Data before any etching, membrane thickness in measurement region $t_m = (47.8 \pm 0.2)$ µm. (Red) data after first etching of 26 mins $Ar/Cl_2$ and 45 mins $O_2$, $t_m = (37.7 \pm 0.2)$ µm. (Green) Data after an additional 30 mins $Ar/Cl_2$ and 138 mins $O_2$ etching, $t_m = (10.1 \pm 0.2)$ µm. (Yellow) Data after an additional 30 mins $Ar/Cl_2$ and 23 mins $O_2$ etching, $t_m = (3.8 \pm 0.2)$ µm. The horizontal clustering of points is a data acquisition artifact.

## VII. CORRELATIONS OF NV CENTER STRAIN AND LINEWIDTH

As discussed in the main text, we are interested to see whether strain regime and measured linewidths are correlated. To this end, we overlay measured broad resonant excitation spectra with simulations of the ZPL transition frequencies calculated from the Hamiltonian of the NV center to determine the local strain environment for individual NVs [8, 9], using the parameters reported in Refs. [10] and [11]: we first fit the position of all peaks in the broad frequency spectrum. We then use two of them as inputs for the $E_x$ and $E_y$ transitions in our model. We then calculate the ground and excited state energies, and compute the allowed transition frequencies between them. We then permute through all combinations of two peaks in the fitted broad spectrum as input for $E_x$ and $E_y$, and use the combination that matches best to the measured spectrum to extract the axial NV strain $\xi_\parallel = (E_x + E_y)/2$ and the transverse NV strain $\xi_\perp = (E_x - E_y)/2$. Fig. 4 (C) shows an example of how we determine the strain regime for an NV center in this way. Out of the 110 distinguishable NV centers studied in this paper, a total of 58 NV centers allowed us to extract a unique strain regime using the method described above. For 24 of these NV centers we characterized the linewidths of two ZPL transitions with a narrow linescan, whereas for the rest of them, only one transition was measured.

As visualized in Fig. 7, we qualitatively find a correlation between axial and transverse strain, and between each of these two strain values and the mirror interface distance. Fig. 8 shows the spectral diffusion (left panels) and dephasing linewidths (right panels) as a function of difference between axial strain of individual NVs and the mean of axial strains of the whole dataset (top panels), axial strain w.r.t. 470.4 GHz (middle panels) and transverse strain (bottom panels). These graphs imply that we cannot explain the observed broadening of linewidths for the final membrane thickness of $t_m = (3.8 \pm 0.2)$ with strain-induced effects.

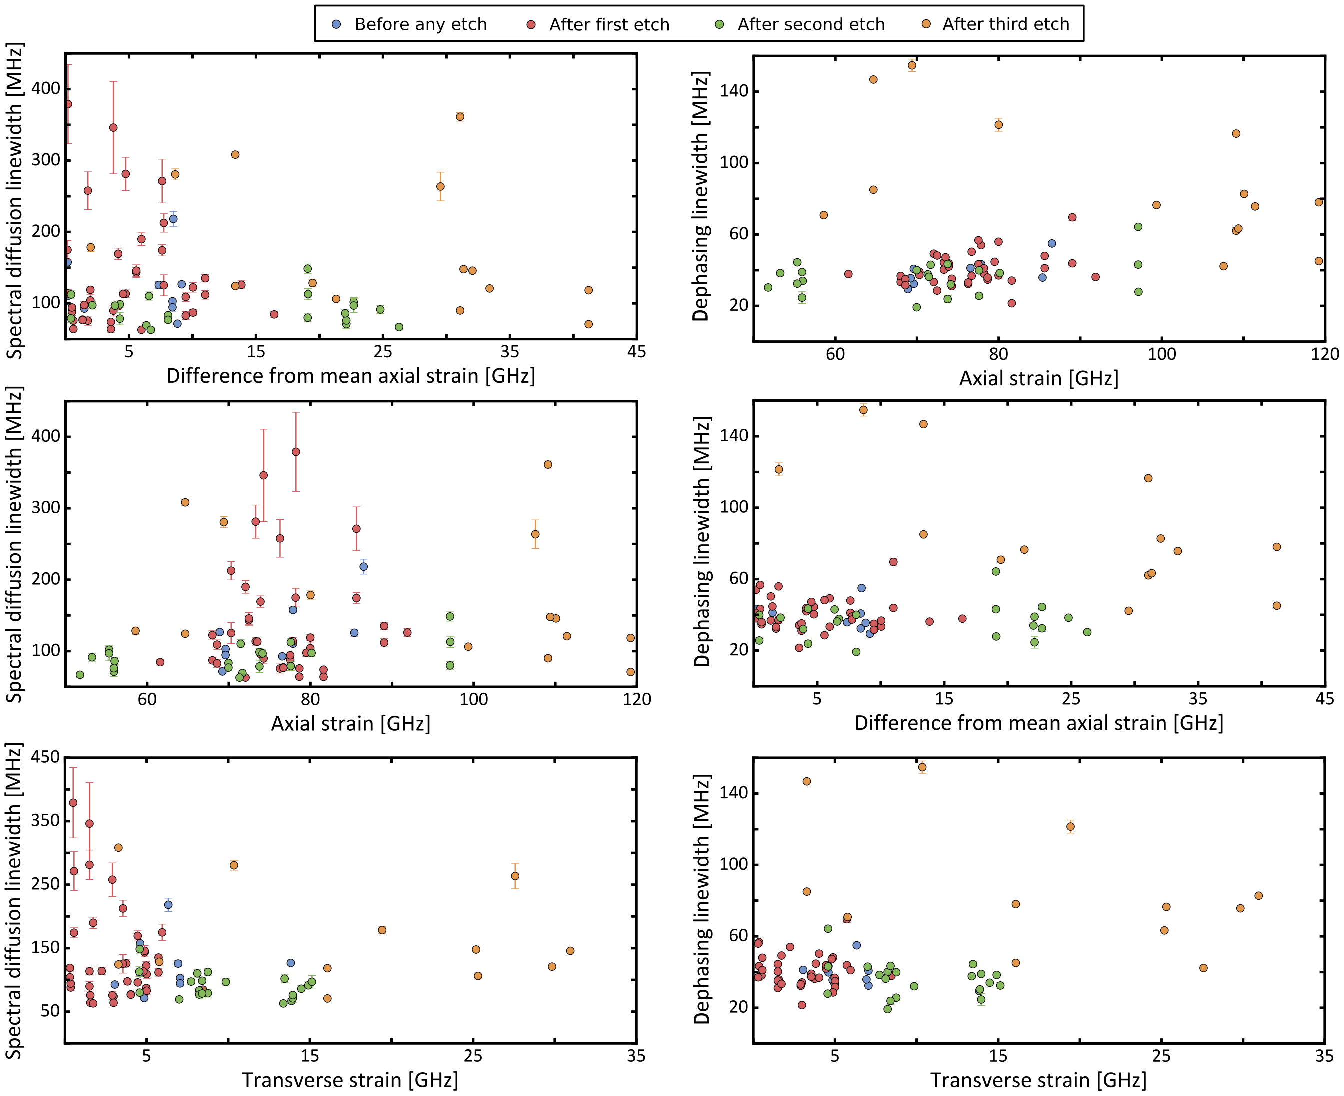


FIG. 8. Spectral diffusion linewidth (left panels) and dephasing linewidths (right panels) of NV centers as a function of transverse and axial strain for different membrane thicknesses. (Top panels) Linewidths as a function of the difference of axial strain of an individual NV from the mean of axial strains of the whole dataset. (Middle panels) Linewidths as a function of axial strain (w.r.t. 470.4 THz). (Bottom panels) Linewidths as a function of transverse strain. The data shows that there is no significant correlation between strain and measured linewidths for our sample. (Blue) Data before any etching, membrane thickness in measurement region $t_m = (47.8 \pm 0.2)$ µm. (Red) data after first etching of 26 mins $Ar/Cl_2$ and 45 mins $O_2$, $t_m = (37.7 \pm 0.2)$ µm. (Green) Data after an additional 30 mins $Ar/Cl_2$ and 138 mins $O_2$ etching, $t_m = (10.1 \pm 0.2)$ µm. (Yellow) Data after an additional 30 mins $Ar/Cl_2$ and 23 mins $O_2$ etching, $t_m = (3.8 \pm 0.2)$ µm.


[1] J. R. Hird and J. E. Field, Proceedings of the Royal Society A: Mathematical, Physical and Engineering Sciences **460**, 3547 (2004).

[2] T. Schuelke and T. A. Grotjohn, Diamond and Related Materials **32**, 17 (2013).

[3] Y. Chu, N. P. De Leon, B. J. Shields, B. Hausmann, R. Evans, E. Togan, M. J. Burek, M. Markham, A. Stacey, A. S. Zibrov, A. Yacoby, D. J. Twitchen, M. Loncar, H. Park, P. Maletinsky, and M. D. Lukin, Nano Letters **14**, 1982 (2014).

[4] S. Bogdanović, M. S. Z. Liddy, S. B. van Dam, L. C. Coenen, T. Fink, M. Lončar, and R. Hanson, APL Photonics **2**, 126101 (2017).

[5] P. Appel, E. Neu, M. Ganzhorn, A. Barfuss, M. Batzer, M. Gratz, A. Tschöpe, and P. Maletinsky, Review of Scientific Instruments **87** (2016).

[6] M. L. Citron, H. R. Gray, C. W. Gabel, and C. R. Stroud, Physical Review A **16**, 1507 (1977).

[7] G. Grynberg, A. Aspect, C. Fabre, and C. Cohen-Tannoudji, *Introduction to Quantum Optics* (Cambridge University Press, Cambridge, 2010).

[8] M. W. Doherty, N. B. Manson, P. Delaney, and L. C. L.

Hollenberg, New Journal of Physics **13** (2011).

[9] J. R. Maze, A. Gali, E. Togan, Y. Chu, A. Trifonov, E. Kaxiras, and M. D. Lukin, New Journal of Physics **13** (2011).

[10] M. W. Doherty, N. B. Manson, P. Delaney, F. Jelezko, J. Wrachtrup, and L. C. L. Hollenberg, Physics Reports **528**, 1 (2013).

[11] L. C. Bassett, F. J. Heremans, D. J. Christle, C. G. Yale, G. Burkard, B. B. Buckley, and D. D. Awschalom, Science **345**, 1333 (2014).
